# Supplementary material for: Fairly Allocating Utility in Constrained Multiwinner Elections
Source: arXiv:2211.12820 source file (2022-11-23)
Supplement: Supplementary file 1 [file appendix.tex]

% {\Huge { Appendix : Paper ID 8678}}

% The references at the end of the main submission is a strict subset of the references at the end of this Appendix. Hence, we conform to the two-page limit as the references at the end of Appendix is at most two pages.

\section{Scoring in Multiwinner Elections}

%Moreover, the conference ACM FAccT, formerly known as FAT*, was established in 2018 to ``bring together researchers and practitioners interested in fairness, accountability, and transparency in socio-technical systems''. 

\section{Proofs}
\label{appedix:proof}

\subsection{Proof of Theorem~\ref{thm:FECuptoxP}}

\subsection{Proof of Theorem~\ref{thm:FECuptoxNP-hard}}

\subsection{Proof of Theorem~\ref{thm:UECNP-hard}}

\subsection{Proof of Corollary~\ref{thm:UECuptoetaNP-hard}}

\subsection{Proof of Theorem~\ref{thm:WECNP-hard}}

\subsection{Proof of Corollary~\ref{thm:WECuptozetaNP-hard}}

\subsection{Proof of Theorem~\ref{thm:DiReManipulation-easy}}

\subsection{Proof of Theorem~\ref{thm:DiReManipulationFEC-hard}}

\subsection{Proof of Theorem~\ref{thm:DiReManipulationUEC-hard}}

\subsection{Proof of Theorem~\ref{thm:DiReManipulationWEC-hard}}

\section{Empirical Analysis}
\label{appendix:empanalysis}
